# Supplementary material for: Effects of additives on oil displacement in nanocapillaries: a mesoscale simulation study
Source: arXiv:2004.10156 source file (2020-04-15)
Supplement: Supplementary file 1 [file PAPER_JMOLLIQ_1_supp_mat.pdf]

# Supplementary Material:

## Effects of additives on oil displacement in nanocapillaries: a mesoscale simulation study

Guilherme C. Q. da Silva<sup>a</sup>, Ronaldo Giro<sup>b</sup>, Bruno A. C. Horta<sup>a</sup>, Rodrigo F. Neumann<sup>b</sup>, Michael Engel<sup>b</sup>, Mathias B. Steiner<sup>b</sup>

<sup>a</sup>*Instituto de Química - Universidade Federal do Rio de Janeiro, Avenida Athos da Silveira Ramos 149 - Bloco A, Sala 609, CEP 21941-909, Rio de Janeiro, RJ, Brazil*

<sup>b</sup>*IBM Research, Av. Pasteur 138/146, CEP 22290-240, Rio de Janeiro, RJ, Brazil*

### 1. Fitting of the MDPD model

This supplementary material displays how the developed MDPD model reproduces the measured data used in the fit. More specifically, Figure S1 and Table S1 compare the calculated properties obtained with the MDPD model and the corresponding reference values used in the fitting procedure. These values were obtained either from experimental values previously reported in the literature or from the all-atom MD simulations performed in this work.

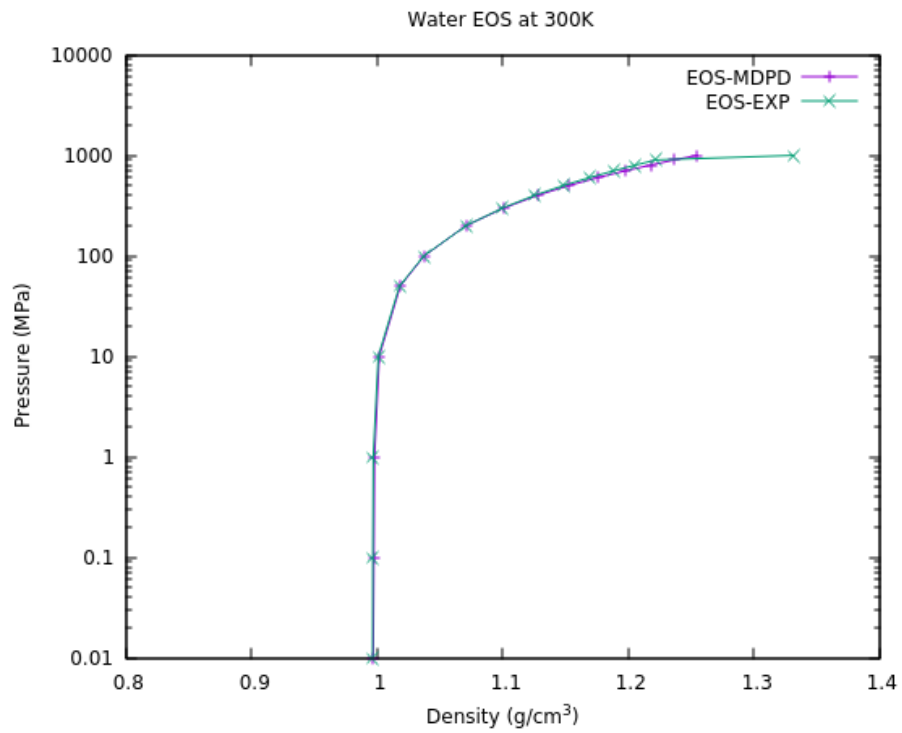

Figure S1: Water PV diagram at 300 K EOS: comparison of the MDPD model and the experimental data reported by Wagner and Pruss (2002) [1].

Table S1: Thermodynamic, dynamic and geometric properties used for fitting the MDPD model developed in this work. Calculated values are reported along with the reference data used as target in the calibration procedure. The reference values correspond to either experimental data previously reported in the literature or data obtained from classical molecular dynamics simulations performed in this work.

|                                                   | MDPD  | Reference                             |
|---------------------------------------------------|-------|---------------------------------------|
| $\rho_{water}$ (g/cm <sup>3</sup> )               | 0.996 | 0.997 <sup>a</sup>                    |
| $\rho_{dodecane}$ (g/cm <sup>3</sup> )            | 0.750 | 0.745 <sup>a</sup>                    |
| $\eta_{water}$ (cP)                               | 0,905 | 0.854 <sup>a</sup>                    |
| $\eta_{dodecane}$ (cP)                            | 1,400 | 1.330 <sup>a</sup>                    |
| $\Gamma_{water-dodecane}$ (mN/m)                  | 54,00 | 52,55 <sup>a</sup>                    |
| $\Gamma_{water-SDS-dodecane}$ near the CMC (mN/m) | 7,4   | 9,1-10,7 <sup>b</sup>                 |
| $\theta^{\circ}_{(water-silica-vapor)}$ (°)       | 20,5  | 21,2 <sup>c</sup>                     |
| $\theta^{\circ}_{(dodecane-silica-vapor)}$ (°)    | 33,0  | 28,0 <sup>c</sup>                     |
| $\theta^0_{(water-silica-dodecane)}$ (°)          | 51,9  | 65,0 <sup>c</sup> / 52,0 <sup>d</sup> |
| $Rg_{(PA-dodecane)}$ (Å) <sup>e</sup>             | 21,0  | 24,7 <sup>c</sup>                     |
| $Rg_{(PA-water)}$ (Å) <sup>e</sup>                | 17,6  | 16,4 <sup>c</sup>                     |
| $Rg_{(PN-dodecane)}$ (Å) <sup>e</sup>             | 7,8   | 8,6 <sup>c</sup>                      |
| $Rg_{(PN-water)}$ (Å) <sup>e</sup>                | 11,7  | 11,6 <sup>c</sup>                     |
| $Rg_{(PAPN-water)}$ (Å) <sup>e</sup>              | 14,1  | 14,0 <sup>c</sup>                     |
| $Rg_{(PA-brine)}$ (Å) <sup>e</sup>                | 11,5  | 7,1 <sup>c</sup>                      |
| $Rg_{(PN-brine)}$ (Å) <sup>e</sup>                | 10,5  | 10,1 <sup>c</sup>                     |

<sup>a</sup> Experimental data from NIST Chemsitry Webbook[2].

<sup>b</sup> Experimental data from Zeppieri *et al.* (2001)[3].

<sup>c</sup> Value obtained with the MD simulations performed in this work.

<sup>d</sup> Experimental data from Bi *et al.* (2004 ) [4].

<sup>e</sup> The subscripts denote the type of polymer in the metioned solvent. PN stands for the non-hydrolized polymer, PA for the fully hydrolized polymer and PAPN the partially hydrolized polymer discussed in the main text.

## References

- [1] W. Wagner, A. Pruß, The IAPWS formulation 1995 for the thermodynamic properties of ordinary water substance for general and scientific use, Journal of Physical and Chemical Reference Data 31 (2) (2002) 387–535. doi:10.1063/1.1461829.  
URL <https://doi.org/10.1063/1.1461829>
- [2] P. Linstrom, Nist chemistry webbook, nist standard reference database 69 (1997). doi:10.18434/T4D303.  
URL <http://webbook.nist.gov/chemistry/>
- [3] S. Zeppieri, J. Rodríguez, A. L. López de Ramos, Interfacial Tension of Alkane + Water Systems, Journal of Chemical & Engineering Data 46 (2001) 1086–1088.
- [4] Z. Bi, W. Liao, L. Qi, Wettability alteration by ctab adsorption at surfaces of sio2 film or silica gel powder and mimic oil recovery, Applied Surface Science 221 (1) (2004) 25 – 31.
